# Supplementary material for: Clustering-based Tile Embedding (CTE): A General Representation for Level Design with Skewed Tile Distributions
Source: arXiv:2210.12789 source file (2022-10-23)
Supplement: Supplementary file 1 [file Appendix.tex]

% Figure \ref{fig:bbcc_outputs} depicts the results of our two-step level generator for the games Bugs Bunny Crazy Castle and those for Genghis Khan are shown in Figure \ref{fig:gk_outputs}. 
% The results consist of both representative good and bad examples of the generated output. Similar to SMB, bad examples of BBCC generation show the presence of unreachable level sections due to the lack of portals/doors, and inconsistency in level structure (Figure \ref{fig:bbcc_outputs}(d)). The dataset levels of Genghis Khan consist of only one pair of town and castle tiles per kevel whereas examples of bad generation (Figure \ref{fig:gk_outputs}(d)), have multiple pairs. The bad level also has randomly placed mountain and forest tiles, instead of the clustered appearance in Figure \ref{fig:gk_outputs}(c) as in the original dataset.

\begin{table*}[!tbh]
\centering
\small
\begin{tabular} {|c| c| c|}
\hline
\textbf{Game} & \textbf{Train} & \textbf{Test} \\
\hline
\textbf{SMB} & 768.92 $\pm$ 140.98 & 743.06 $\pm$ 101.67 \\
\hline
\textbf{Genghis Khan} & 39.32 $\pm$ 3.93 & 40.98 $\pm$ 5.18 \\
\hline
\textbf{BBCC} & 190.03 $\pm$ 22.27 & 210.98 $\pm$ 20.75 \\
\hline
\end{tabular}
\caption{Edit Distance between the generated cluster representations and train-test split of the dataset. The difference between training and testing values is not statistically significant. This demonstrates that the model is not overfitting.}
\label{table:edit_distance}
\end{table*}

% \begin{table}[!tbh]
% \centering
% \small
% \begin{tabular} {|c| c c| c|}
% \hline
%  & 
% \multicolumn{2}{c|}{Clustering} & Translation \\[1.0ex]
% & Number of & Silhouette &  SSIM\\
% & Clusters & Score &\\
% \hline
% \hline
% SMB & 11 & 0.91 & 0.9976 $\pm$ 0.0014\\[0.5ex]
% \hline
% Genghis Khan & 8 & 0.39 & 0.8689 $\pm$ 0.01\\[0.5ex]
% \hline
% BBCC & 24 & 0.53 & 0.9792 $\pm$ 0.0079\\[0.5ex]
% \hline
% \end{tabular}
% \caption{Evaluating Clustering and Translator modules}
% \label{table:eval_clus_translation}
% \end{table}

\begin{figure*}[tbh]
    \centering
     \includegraphics[width=6.5in]{LaTeX/Figures/smb_more_outputs.drawio.png}
     \caption{More Examples of SMB Level Generation}
     \label{fig:more_smb_outputs}
\end{figure*}

\begin{figure*}[tbh]
    \centering
     \includegraphics[width=6.5in]{LaTeX/Figures/bbcc_outputs.drawio (2).png}
     \caption{Level Generation for Bugs Bunny Crazy Castle : (a) Dataset level and its Corresponding translation output with differences highlighted in yellow (b) Examples of good generation output (c) Examples of bad generation output. Unlike good examples of generation in shown in (b), bad examples in (c) show the presence of unreachable level sections due to the lack of portals/doors, and inconsistency in level structure.}
     \label{fig:bbcc_outputs}
\end{figure*}

\begin{figure*}[tbh]
    \centering
     \includegraphics[width=6in]{LaTeX/Figures/gk_outputs.drawio (3).png}
     \caption{Level Generation for Genghis Khan : (a) Dataset level (b) Corresponding translation output with differences highlighted in red (c) Example of good generation output (b) Example of bad generation output. The dataset levels of Genghis Khan consist of only one pair of town and castle tiles per level whereas examples of bad generation (c), have multiple pairs. The bad level also has randomly placed mountain and forest tiles, instead of the clustered appearance in (b) as in the original dataset.}
     \label{fig:gk_outputs}
\end{figure*}
